# Supplementary material for: Diffusion Models and Representation Learning: A Survey
Source: arXiv:2407.00783 source file (2024-06-30)
Supplement: Supplementary file 1 [file 61_appendix.tex]

\section{Appendix}

\section{Cover Letter}

Dear Editor:

  We would like to submit our research entitled "Diffusion Models and Representation Learning:
A Survey" for consideration by TPAMI.
  
  This manuscript is an extension of our previous conference paper [1]. In the conference paper, the proposed algorithms only apply to the matrix square root. For the inverse square root, we have to compute the linear system or the matrix inverse, which is not efficient enough. In this manuscript, we extend our algorithm to the case of inverse square root with a marginally higher computational cost. Moreover, we validate our methods in four more real-world computer vision applications.
  
  We believe that this manuscript is appropriate for publication by TPAMI because it concerns an important computational method of a technique that is widely used in computer vision and deep learning.
  
  Thank you for your consideration of this manuscript.
  
Sincerely,
  
Michael Fuest, Pingchuan Ma, Ming Gui, Johannes Schusterbauer, Vincent Tao Hu, Bj ̈orn Ommer
